# Supplementary material for: A Transformation-based Implementation for CLP with Qualification and Proximity
Source: arXiv:1201.5418 source file (2012-01-25)
Supplement: Supplementary file 1 [file JAppendix.tex]

% ----
% Appendix: Syntax of SQCLP Programs
% ----
\section{Syntax of SQCLP Programs}
\label{sec:syntax-programs}

Terminals are shown enclosed between single quotes, non-terminal are written in capital letters and lexical elements in lower case letters. These lexical elements are the following:

\begin{itemize}
\item
{\tt id:} Any lower case letter ({\tt a}--{\tt z}) followed by any combination of lower/upper case letters ({\tt a}--{\tt z}{\tt A}--{\tt Z}), digits ({\tt 0}--{\tt 9}), underscores (\_) and apostrophes (').
\item
{\tt sstring:} Any sequence of characters enclosed between single quotes (`').
\item
{\tt dstring:} Any sequence of characters enclosed between double quotes (``'').
\item
{\tt op:} Any sequence of the following characters: {\tt aaa}.
\item
{\tt nop:} An {\tt op} element enclosed between parentheses (without spaces!).
\item
{\tt var:} Similar to {\tt id}s but starting with either an upper case letter ({\tt A}--{\tt Z}) or an underscore (\_).
\item
{\tt integer:} Any sequence of digits ({\tt 0}--{\tt 9}).
\item
{\tt float:} Two {\tt integer}s separated by one dot (.). Note that in this context, and for the following syntax, {\tt integer}s and {\tt float}s are syntactically different elements and therefore floats must be written with the decimal dot. That is, one will have to write {\tt `3'} for the integer 3, and {\tt `3.0'} for the float 3.
\end{itemize}

The syntax for SQCLP programs is:

\begin{verbatim}
% SQCLP Program
PROGRAM := `{' (DIRECTIVES `;')? CLAUSES? `}'

% Directives
DIRECTIVES := DIRECTIVE (`;' DIRECTIVE)*
DIRECTIVE := `#' NAME DTERM*
DTERM := LITERAL | NAME | `(' DTERM (`,' DTERM)* `)'

% Clauses
CLAUSES := CLAUSE (`;' CLAUSE)*
CLAUSE := ATOM BODY
BODY := `<--' (BODYATOM (`,' BODYATOM)*)?
      | `<-' QVAL `-' (BODYATOM (`,' BODYATOM)*)?
BODYATOM := ATOM (`#' ANNOTATION)? | PRIM (`#' ANNOTATION)?
ANNOTATION := `?' | QVAL

% Atoms
ATOM := NAME (`(' TERM (`,' TERM)* `)')?
PRIM := `(' PRIM `)'
      | TERM `=' TERM op TERM
      | TERM op TERM (`=' TERM)?

% Terms
TERM := var
      | LITERAL
      | `[]' | `[' TERM (`,' TERM)* (`|' TERM)? `]'
      | `()' | `(' TERM `,' TERM (`,' TERM)* `)'
      | NAME (`(' TERM (`,' TERM)* `)')?
      | `-' TERM
      | `(' TERM `)'
NAME := id | sstring | nop
LITERAL := integer | float | dstring
\end{verbatim}

Note that in the previous grammar the non-terminal {\tt QVAL} has not been defined. The reason for this is because this non-terminal is dependent on the specific qualification domain in use: it will be either a {\tt float} (for domains {\tt u} and {\tt w}) or a tuple of {\tt float}s (for any product domain as {\tt (u,w)}).

Two directives can be defined in SQCLP programs. One for specifying the particular qualification domain used, and another one for linking a proximity relation to be used with the given SQCLP program. These two directives are defined in the following way:
\begin{verbatim}
    # qdom u
    # prox `Proximity'
\end{verbatim}
where {\tt u} means that the qualification domain to be used is $\U$ and {\tt `Proximity'} that a file {\em `Proximity.qclp'} should exist containing a proximity relation. One could also write {\tt w} for the qualification domain $\W$, and any tuple of those two for the product domain they will conform, i.e. {\tt (u,w)} for $\U\!\otimes\!\W$. While the {\tt qdom} directive is mandatory and should be specified in every SQCLP program, the {\tt prox} directive is optional, and if not provided, $\sid$ will be assumed as the proximity relation.

% ----
% Appendix: Syntax of SQCLP Goals
% ----
\section{Syntax of SQCLP Goals}
\label{sec:syntax-goals}
